# Supplementary material for: GenCLIP: Generalizing CLIP Prompts for Zero-shot Anomaly Detection
Source: arXiv:2504.14919 source file (2025-04-21)
Supplement: Supplementary file 1 [file appendix.tex]

\documentclass[10pt,twocolumn,letterpaper]{article}

%%%%%%%%% PAPER TYPE  - PLEASE UPDATE FOR FINAL VERSION
% \usepackage{iccv}              % To produce the CAMERA-READY version
\usepackage[review]{iccv}      % To produce the REVIEW version
\usepackage{tabularx}
\usepackage{pifont}
\usepackage{adjustbox}
\usepackage{multirow}
\usepackage{booktabs}
\usepackage{colortbl}
\usepackage{multicol}
\usepackage[nobalance]{flushend}
\usepackage{setspace}

% \usepackage[pagenumbers]{iccv} % To force page numbers, e.g. for an arXiv version

% Import additional packages in the preamble file, before hyperref
\input{preamble}

% It is strongly recommended to use hyperref, especially for the review version.
% hyperref with option pagebackref eases the reviewers' job.
% Please disable hyperref *only* if you encounter grave issues, 
% e.g. with the file validation for the camera-ready version.
%
% If you comment hyperref and then uncomment it, you should delete *.aux before re-running LaTeX.
% (Or just hit 'q' on the first LaTeX run, let it finish, and you should be clear).
\definecolor{iccvblue}{rgb}{0.21,0.49,0.74}
\usepackage[pagebackref,breaklinks,colorlinks,allcolors=iccvblue]{hyperref}

%%%%%%%%% PAPER ID  - PLEASE UPDATE
 % *** Enter the Paper ID here

%%%%%%%%% TITLE - PLEASE UPDATE
\title{Appendix for GenCLIP}

%%%%%%%%% AUTHORS - PLEASE UPDATE
\author{
Donghyeong Kim \quad Chaewon Park \quad Suhwan Cho Hyeonjeong Lim Minseok Kang Sangyoun Lee\\
Yonsei University, Seoul, Korea \\
{\tt\small \{2donghyung87, chaewon28, jeonggg119, louis0503, syleee\}@yonsei.ac.kr, suhwanx@gmail.com}
}

\begin{document}
\maketitle
\renewcommand{\thesection}{\Alph{section}} % This resets the section numbering to A, B, C, etc.

\maketitle
\renewcommand{\thesection}{\Alph{section}} % This resets the section numbering to A, B, C, etc.

\input{sec/Details}
\input{sec/Analysis}

% \clearpage

% \newpage

% {
%     \small
%     \bibliographystyle{ieeenat_fullname}
%     \bibliography{main}
% }

% \end{document}

\clearpage
\newpage
\begingroup
\setstretch{1.0}
\normalsize
{
    \small
    \bibliographystyle{ieeenat_fullname}
    \setlength{\bibsep}{0pt}
    \setlength{\itemsep}{0.2\baselineskip}
    \begin{onecolumn}
    \bibliography{main}
    \end{onecolumn}
}
\endgroup

\input{sec/Details}
\input{sec/Analysis}

% \clearpage

% \newpage

% {
%     \small
%     \bibliographystyle{ieeenat_fullname}
%     \bibliography{main}
% }

% \end{document}

\clearpage
\newpage
\begingroup
\setstretch{1.0}
\normalsize
{
    \small
    \bibliographystyle{ieeenat_fullname}
    \setlength{\bibsep}{0pt}
    \setlength{\itemsep}{0.2\baselineskip}
    \begin{onecolumn}
    \bibliography{main}
    \end{onecolumn}
}
\endgroup

\end{document}
